# Supplementary material for: Superlinear Precision and Memory in Simple Population Codes
Source: arXiv:2008.00629 ancillary file (2020-08-03)
Supplement: Supplementary file 1 [file supplementary.pdf]

# Supplementary Material

Here, we present a heuristic derivation of the scaling relation for optimal tuning curve width in the presence of a nonzero baseline firing rate. We then verify the results using numerical simulations.

## 1 Threshold error for nonzero baseline

We consider $N$ independent Poisson neurons that respond to 1D periodic stimulus $\phi \in [0, 2\pi]$. Their preferred stimulus values $\phi_i$ are evenly distributed such that the inter-neuronal spacing is $d\phi = 2\pi/N$. Their tuning curves are given by:

$$\lambda_i = \lambda_{max} \left[(1-\epsilon) f_i(\sigma, |\phi - \phi_i|) + \epsilon\right] \tag{S1}$$

where we now assume that $0 < \epsilon \ll 1$ gives rise to a small but nonzero baseline firing rate, $\lambda_{max}\epsilon$.

We divide the neurons into $n_{group} = 2\pi/2\sigma = \pi/\sigma$ groups such that each group covers a non-overlapping stimulus interval of width $2\sigma$ and contains $N_\alpha = 2\sigma/ds = N\sigma/\pi$ neurons. During the experiment, each particular true stimulus value will fall on the interval covered by one particular group, denoted the *local group* (see Figure 1). Let $X$ be the total number of spikes fired by all the neurons in the local group in response to the stimulus during the time interval $T$. For independent Poisson neurons, $X$ will also be Poisson distributed with rate parameter $\Lambda T$ where $\Lambda$ is the sum of the firing rates of the neurons in the local group. Without loss of generality, assume that the true stimulus value is $\phi = 0$. We can compute $\Lambda$ by summing over (S1) for neurons with centers $\frac{2\pi}{N} i, \quad i = -N\sigma/2\pi, \ldots, N\sigma/2\pi$:

$$\Lambda = \lambda_{max} \sum_{i=-N\sigma/2\pi}^{+N\sigma/2\pi} \left[(1-\epsilon) f_i(\sigma, |\phi - \phi_i|) + \epsilon\right] \tag{S2}$$

$$\tag{S3}$$

In the large $N$ limit, we can convert the summation into an integral and possibly give an analytic expression for $\Lambda$ depending on the exact form of the tuning curves. Below, we will assume that this computation can be done and work with average firing rate $\lambda \coloneqq \Lambda/N_\alpha$ for the neurons in the local group. Thus, we have:

$$X \sim Poiss(N_\alpha \lambda T) = Poiss\left(\frac{N\sigma\lambda T}{\pi}\right) \tag{S4}$$

In the zero baseline case, any neuron outside this local group will have negligible firing rate and so the threshold error will occur only when $X = 0$, corresponding to non-response. For the nonzero baseline case however, non-response is unlikely since all neurons outside the local group have non-negligible firing rate $b \coloneqq \lambda_{max}\epsilon$ and instead threshold error will typically occur when a

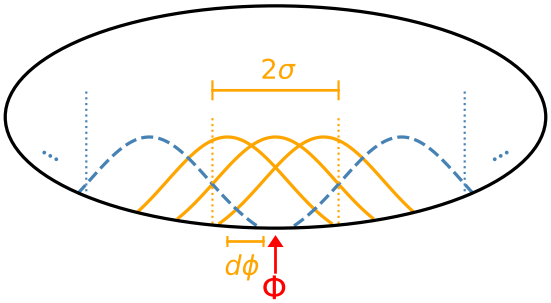


Figure 1: Schematic of the coding network. Ellipse represents the ring of neurons composing the network. Tuning curves corresponding to the local group of neurons with respect to the presented stimulus value $\Phi$ has been highlighted in orange (solid), while two adjacent neurons belonging to non-local groups are colored blue (dashed). $ds$ is the interneuronal spacing and $\sigma$ is the tuning curve width.

*non-local group* of neurons fires more spikes than the local group. Let $Y_\alpha$ be the total number of spikes fired by all the neurons in the $\alpha$th non-local group. As before, $Y_\alpha$ will be Poisson distributed with rate parameter $BT$ where $B = N_\alpha b$ is the total baseline firing rate of the group. We thus have:

$$Y_\alpha \sim Poiss(N_\alpha bT) = Poiss\left(\frac{N\sigma bT}{\pi}\right) \tag{S5}$$

In conclusion, the threshold error in the nonzero baseline case occurs when $Y_\alpha > X$ for at least one non-local group $\alpha$.

## 2 Threshold error probability

In this section, we derive the probability $p_{th}$ that threshold error will occur in the nonzero baseline case, i.e. the probability that $Y_\alpha > X$ for at least one $\alpha$.

First, for analytical tractability, we approximate the Poisson distribution with a Gaussian. That is,

$$X \sim N\left(\frac{N\sigma\lambda T}{\pi}, \frac{N\sigma\lambda T}{\pi}\right) \tag{S6}$$

$$Y_\alpha \sim N\left(\frac{N\sigma bT}{\pi}, \frac{N\sigma bT}{\pi}\right) \tag{S7}$$

The condition under which this is appropriate is $N_\alpha\lambda T, N_\alpha bT \gg 0$. This is assured for large $N$ limit if $\sigma$ decreases more slowly than $1/N$, i.e. $N\sigma = \omega(1)$. As in the main text, we will see that the optimal width scaling that we derive is consistent with this assumption.

To compare two Gaussian variables $X \sim N(\mu_x, \sigma_x^2)$ and $Y \sim N(\mu_y, \sigma_y^2)$, we can use the following formula:

$$P(X < Y) = \frac{1}{2}\text{erfc}\left(\frac{\mu_x - \mu_y}{\sqrt{2(\sigma_x^2 + \sigma_y^2)}}\right) \tag{S8}$$

where $\text{erfc}(x) = 1 - \text{erf}(x) = \frac{2}{\sqrt{\pi}}\int_x^\infty e^{-t^2}dt$ is the complementary error function.

Making appropriate substitutions, the probability that a particular non-local group fires more spikes than the local group is:

$$P(X < Y_\alpha) = \frac{1}{2}\text{erfc}\left(\sqrt{\frac{N\sigma\lambda T}{2\pi}}\frac{1 - b/\lambda}{\sqrt{1 + b/\lambda}}\right) \tag{S9}$$

Note that the right hand side is independent of index $\alpha$, as all non-local neurons have been assumed to have the identical baseline firing rate.

We now write the expression for the actual probability of getting threshold error, which is exactly the probability that $X < Y_\alpha$ for some $\alpha$:

$$p_{th} \coloneqq P(\exists\alpha : X < Y_\alpha) = P\left(\bigcup_{\alpha=1}^{n_{group}}\{X < Y_\alpha\}\right) \tag{S10}$$

While it is possible to write out the right hand side in terms of nested integrals over Gaussians, no closed-form expression can be obtained and only the numerical evaluation is tractable. Instead, we use the union bound on the threshold error probability:

$$\begin{aligned} p_{th} &= P\left(\bigcup_{\alpha=1}^{n_{group}}\{X < Y_\alpha\}\right) & \text{(S11)}\\ &\leq \sum_{\alpha=1}^{n_{group}} P(X < Y_\alpha) & \text{(S12)}\\ &= \frac{\pi}{2\sigma}\text{erfc}\left(\sqrt{\frac{N\sigma\lambda T}{2\pi}}\frac{1 - b/\lambda}{\sqrt{1 + b/\lambda}}\right) & \text{(S13)}\\ &\eqqcolon p'_{th} & \text{(S14)}\end{aligned}$$

where we substituted in (S9) to get (S13).

In subsequent sections, we use the upper bound $p'_{th}$ in place of the actual threshold error probability $p_{th}$ to derive the scaling relation for the optimal tuning width. Since this is a pessimistic approximation (i.e. we assume that catastrophic non-local errors occur more often than is actually the case), we expect the true error and optimal width scalings to decrease faster than the results we derive below. That will be sufficient for our purpose.

Before proceeding to derive the optimal tuning width, we use the assumption already made that $N\sigma = \omega(1)$ to simplify the expression for $p'_{th}$. We also need the following fact:

$$\lim_{x\to\infty}\text{erfc}(x) = \frac{e^{-x^2}}{x\sqrt{\pi}} \tag{S15}$$

Then, in the large $N$ limit, we get:

$$\begin{aligned} p'_{th} &= \frac{\pi}{2\sigma}\text{erfc}\left(\sqrt{\frac{N\sigma\lambda T}{2\pi}}\frac{1 - b/\lambda}{\sqrt{1 + b/\lambda}}\right) & \text{(S16)}\\ &\simeq \frac{\pi}{\sqrt{2N\sigma^3\lambda T}}\frac{\sqrt{1 + b/\lambda}}{1 - b/\lambda}e^{-\frac{N\sigma\lambda T}{2\pi}\frac{(1-b/\lambda)^2}{1+b/\lambda}} & \text{(S17)}\end{aligned}$$

Also note that $p'_{th} \ll 1$ in the same limit.

# 3 Optimal tuning curve width

We take from the main text the following form for the mean squared error (MSE):

$$MSE = \frac{\sigma}{\alpha N}(1 - p'_{th}) + \beta p'_{th} \simeq \frac{\sigma}{\alpha N} + \beta p'_{th}, \text{as } N \to \infty \tag{S18}$$

where $\alpha = \alpha(T, \lambda)$ is a prefactor for the local error given by FI and $\beta = \pi^2/3$ is the mean-squared error in the case of random guessing over the circle. The latter is still the appropriate form for the threshold error for the nonzero baseline case since in such an event the non-local group that fired more spikes than the local group could have been located anywhere along the stimulus space.

Now, we take the derivative to find the optimal tuning curve width, $\sigma^*$:

$$0 \stackrel{!}{=} \left.\frac{\partial MSE}{\partial \sigma}\right|_{\sigma=\sigma^*} = \frac{1}{\alpha N} + \beta \left.\frac{\partial p'_{th}}{\partial \sigma}\right|_{\sigma=\sigma^*} \tag{S19}$$

It is straightforward to calculate the derivative of $p'_{th}$:

$$\frac{\partial p'_{th}}{\partial \sigma} = -\left[\frac{3\pi}{\sqrt{8\lambda T}} \frac{1}{\sqrt{N\sigma^5}} + \sqrt{\frac{\lambda T}{8}} \frac{(1 - b/\lambda)^2}{1 + b/\lambda} \sqrt{\frac{N}{\sigma^3}}\right] e^{-\frac{\lambda T}{2\pi} \frac{(1-b/\lambda)^2}{1+b/\lambda} N\sigma} \tag{S20}$$

For our purposes, we are only concerned with the parameters $\sigma$ and $N$. To simplify notation, define the following shorthands:

$$c_0 \coloneqq \frac{1}{\alpha} \tag{S21}$$

$$c_1 \coloneqq \frac{3\pi\beta}{\sqrt{8\lambda T}} \tag{S22}$$

$$c_2 \coloneqq \beta \sqrt{\frac{\lambda T}{8}} \frac{(1 - b/\lambda)^2}{1 + b/\lambda} \tag{S23}$$

$$c_3 \coloneqq \frac{\lambda T}{2\pi} \frac{(1 - b/\lambda)^2}{1 + b/\lambda} \tag{S24}$$

Then, we can write (S19) as:

$$\frac{c_0}{N} = \left[c_1 \frac{1}{\sqrt{N\sigma^5}} + c_2 \sqrt{\frac{N}{\sigma^3}}\right] e^{-c_3 N\sigma} \tag{S25}$$

$$= \left[c_1 \frac{1}{N\sigma} \sqrt{\frac{N}{\sigma^3}} + c_2 \sqrt{\frac{N}{\sigma^3}}\right] e^{-c_3 N\sigma} \tag{S26}$$

$$\simeq c_2 \sqrt{\frac{N}{\sigma^3}} e^{-c_3 N\sigma} \tag{S27}$$

The last line follows from $N\sigma = \omega(1)$.

Taking logarithm of both sides, we get:

$$\log c_0 - \log N \simeq \log c_2 + \frac{1}{2} \log N - \frac{3}{2} \log \sigma - c_3 N\sigma \tag{S28}$$

$$\implies c_3 N\sigma \simeq \log \frac{c_2}{c_0} + \frac{3}{2} \log N + \frac{3}{2} \log \frac{1}{\sigma} \tag{S29}$$

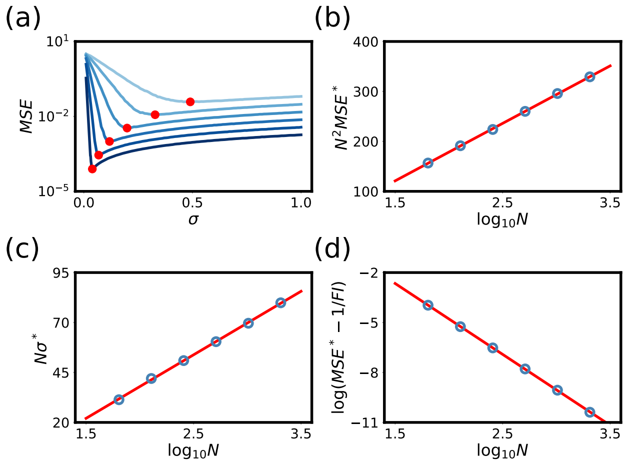


Figure 2: (a) MSE versus tuning curve width obtained from simulations with maximum likelihood decoding for system sizes $N = 64, 128, 256, 512, 1024, 2048$ (top to bottom). Unlike for the case described in the main text, there is a nonzero baseline firing rate (10% of the maximum of the original Gaussian; specifically, we set $\lambda_{max} = 1.1$ and $\epsilon \approx 0.09$ in ). Dots indicate the minima (MMSE). (b) Plot of $N^2MSE^*$ versus $\log N$. (c) Plot of $N\sigma^*$ versus $\log N$. (d) Plot of $\log(MSE^* - 1/FI)$ versus $\log N$. The extra error beyond the local FI contribution behaves as predicted.

Clearly, $N\sigma = \omega(1)$ implies $1/\sigma = o(N)$. Thus, in the large $N$ limit, only the $\log N$ term becomes significant on the right hand side. It then follows that:

$$\sigma \simeq \frac{3}{2c_3}\frac{\log N}{N} \tag{S30}$$

Thus, the optimal tuning width has the scaling $\sim \log N/N$. However, recall that we used the upper bound for $p_{th}$ for deriving this. In actuality, because the threshold error is less likely to occur, it is possible that the optimal tuning width scaling would be narrower. $\sim \log N/N$ represents the upper bound for the scaling. On the other hand, $\sim \log N/N$ is the optimal tuning width for the zero baseline case as derived in the main text. Since the presence of baseline increases the threshold error probability, we expect the optimal tuning width with baseline to be no narrower than this. From these considerations we can deduce that the optimal tuning scaling for the nonzero baseline case is in fact $\sim \log N/N$ and thus coincides with the zero baseline case.

# 4 Numerical results

In previous sections, we presented heuristic arguments to demonstrate why it is plausible that the results obtained in the main text would generalize to the nonzero baseline case. To augment the argument with data, we turned to numerical simulations.

Figure 2 shows the results of maximum likelihood decoding simulations with nonzero baseline firing rate. They are comparable to the corresponding results obtained using zero baseline (see main text), corroborating that the nonzero baseline firing rate does not significantly affect the general scaling relation.
